# Supplementary material for: Relativistic correction scheme for core-level binding energies from $GW$
Source: arXiv:2005.13465 ancillary file (2020-06-12)
Supplement: Supplementary file 1 [file supporting_information.pdf]

# Supporting Information:

## Relativistic correction scheme for core-level binding energies

### from $GW$

Levi Keller,<sup>\*,†</sup> Volker Blum,<sup>‡</sup> Patrick Rinke,<sup>†</sup> and Dorothea Golze<sup>†</sup>

<sup>†</sup>*Department of Applied Physics, Aalto University, Otakaari 1, FI-02150 Espoo, Finland*

<sup>‡</sup>*Department of Mechanical Engineering and Materials Science, Duke University, Durham, North Carolina  
27708, USA*

E-mail: levi.keller@aalto.fi

## 1 Non-spherical and spherical atomic solutions

In deriving the element specific relativistic correction for the free atoms, we employ the fractional occupation approximation in order to exploit spherical symmetry. For open shell systems, the true ground-state is  $2S+1$ -fold degenerate, where  $S$  is the total spin. This nonspherical solution breaks the spin-degeneracy of the  $1s$  shell. In order to quantify how coarse an approximation the fractional approximation introduces, we compare the  $1s$  eigenvalues of the spherical solution with another in which  $M_S$  is constrained. The results, shown in Table S1, indicate that the difference is small compared to the magnitude of the relativistic correction employed. Some cancellation of this error is expected, as the relativistic correction entail difference of terms both containing it. The results of the molecular calculation with DIRAC (Figure 2(c) in the main article) bear this out, as the relativistic correction for the  $1s$  eigenvalues of closed shell molecules differ from the atomic value calculated within the fractional occupation approximation by less than 0.01 eV for all but one state, which barely exceeds it. This value is smaller than the  $\Delta_{\text{spher}}$  of Table S1.

**Table S1:** Atomic  $1s$  DFT eigenvalues  $\epsilon_{1s,\text{at}}$  obtained at the non-relativistic Schrödinger Kohn-Sham level with the LDA functional employing NAOs of *tier2* quality.<sup>1</sup> Calculations for a free neutral atom. Without intervention, a spherical solution is obtained with fractional occupation numbers. For the second-row, elements B, C, O and F are affected. Enforcing integer occupation numbers, a non-spherical ground state solution is found for these elements, which is lower in energy. The difference between spherical and non-spherical solution is  $\Delta_{\text{spher}} = |\epsilon_{1s,\text{at}}^{\text{spherical}} - \epsilon_{1s,\text{at}}^{\text{non-spherical}}|$ . “up” and “down” refer to the spin channels.

| atomic level | spherical |         | non-spherical |         | $\Delta_{\text{spher}}$ |      |
|--------------|-----------|---------|---------------|---------|-------------------------|------|
|              | up        | down    | up            | down    | up                      | down |
| B1s          | -178.56   | -178.21 | -178.53       | -178.19 | 0.03                    | 0.02 |
| C1s          | -270.47   | -269.51 | -270.47       | -269.52 | 0.00                    | 0.02 |
| O1s          | -510.67   | -509.18 | -510.66       | -509.15 | 0.01                    | 0.04 |
| F1s          | -658.54   | -657.69 | -658.58       | -657.70 | 0.04                    | 0.01 |

## 2 Basis set extrapolation

It has been observed that *GW* methods, like correlated electronic structure methods, converge slowly with respect to the number of basis functions.<sup>2–5</sup> Unlike in plane-wave codes, where the number of basis functions can be continuously increased, when using local basis sets, a limited number of basis sets of fixed size are available, and extrapolation techniques are necessary to attain the complete basis set limit. The Dunning correlation consistent (cc-pVnZ, n=3-6) family of basis sets were designed to facilitate the smooth convergence of correlated methods to the complete basis set limit.<sup>6,7</sup> The basis-set design strategies of Dunning and coworkers have since been adapted in various ways. These include augmentation by additional diffuse functions to better describe weak bonds and some properties (aug-cc-pVnZ),<sup>8</sup> the addition of outer core correlating functions designed to optimize the core-valence correlation energy (cc-pCVnZ)<sup>9</sup> and the adaptation to numerical atom-centered orbitals (NAO-VCC-nZ).<sup>10</sup> To the best of our knowledge, no systematic study has been performed of the performance of these various basis set series in conjunction with the *GW* method.

We examine the convergence behavior of these basis sets by looking at the mean and absolute mean error by species for the triple- $\zeta$  (3Z), quadruple- $\zeta$  (4Z) and extrapolated  $\text{evGW}_0$  quasiparticle energies (Figure S1). We find that the results depend on the basis set family. The cc-pCVnZ have an unusually large MAE/ME ratio, indicating that the errors are widely distributed and non-systematic. In addition, the errors increase inconsistently for different species, even trending in the opposite direction sign-wise. The NAO-VCC-nZ family performs in a more systematic way, but overestimates the binding energy. The overestimation indicates that the number of core functions might be too small. Similar effects of basis set incompleteness due to missing core functions have been reported for core-level spectra from  $\Delta\text{SCF}$ <sup>11,12</sup> or coupled cluster-based methods.<sup>13</sup> The cc-pVnZ and aug-cc-pVnZ show very similar performance. Both underestimate the 1s binding energies. The mean error is consistently improved when increasing the virtual space, i.e., when increasing the basis set size. We therefore employ the cc-pVnZ basis sets because they allow for a reliable extrapolation to the complete basis set limit.

## 3 Basis sets for relativistic calculations

Nonrelativistic basis sets are not optimally suited for describing the more compact pseudo- and scalar-relativistic orbitals. Nevertheless, in order to facilitate comparison with the non-relativistic calculation, we require a similar level of accuracy in the description of the virtual spectrum. As the numerically-tabulated NAO-VCC-nZ basis set series<sup>10</sup> are fitted to the bare atomic orbitals calculated with the aZORA Hamiltonian, they are well-suited to describe scalar-relativistic orbitals. With the NAO-VCC-5Z values as a reference, we examine the convergence of the 1s Kohn-Sham eigenvalues in Table S2 to estimate the magnitude of the basis set incompleteness error in the aZORA calculations. While the NAOs are converged to within a few meV already at the 4Z level, the cc-pVnZ series reaches a similar level of accuracy only at the 6Z level.

**Table S2:** Mean, absolute mean and maximum deviation of the Kohn-Sham 1s eigenvalues ( $\Delta\epsilon_{1s}$ ) for the 65 core excitations. Deviations are defined as  $\Delta(\text{Basis set}) = \epsilon_{1s}(\text{Basis set}) - \epsilon_{1s}(\text{NAO-VCC-5Z})$ . NAO-VCC-nZ is abbreviated as NAO-nZ

| $n =$     | $\Delta(\text{NAO-VCC-}n\text{Z})$ |       |        | $\Delta(\text{cc-pV}n\text{Z})$ |       |       |       |       |
|-----------|------------------------------------|-------|--------|---------------------------------|-------|-------|-------|-------|
|           | 2                                  | 3     | 4      | D                               | T     | Q     | 5     | 6     |
| mean      | -0.090                             | 0.003 | -0.001 | -0.212                          | 0.063 | 0.134 | 0.037 | 0.009 |
| mean abs. | 0.105                              | 0.016 | 0.007  | 0.231                           | 0.065 | 0.134 | 0.037 | 0.011 |
| max abs.  | 0.301                              | 0.099 | 0.031  | 0.437                           | 0.409 | 0.352 | 0.105 | 0.029 |

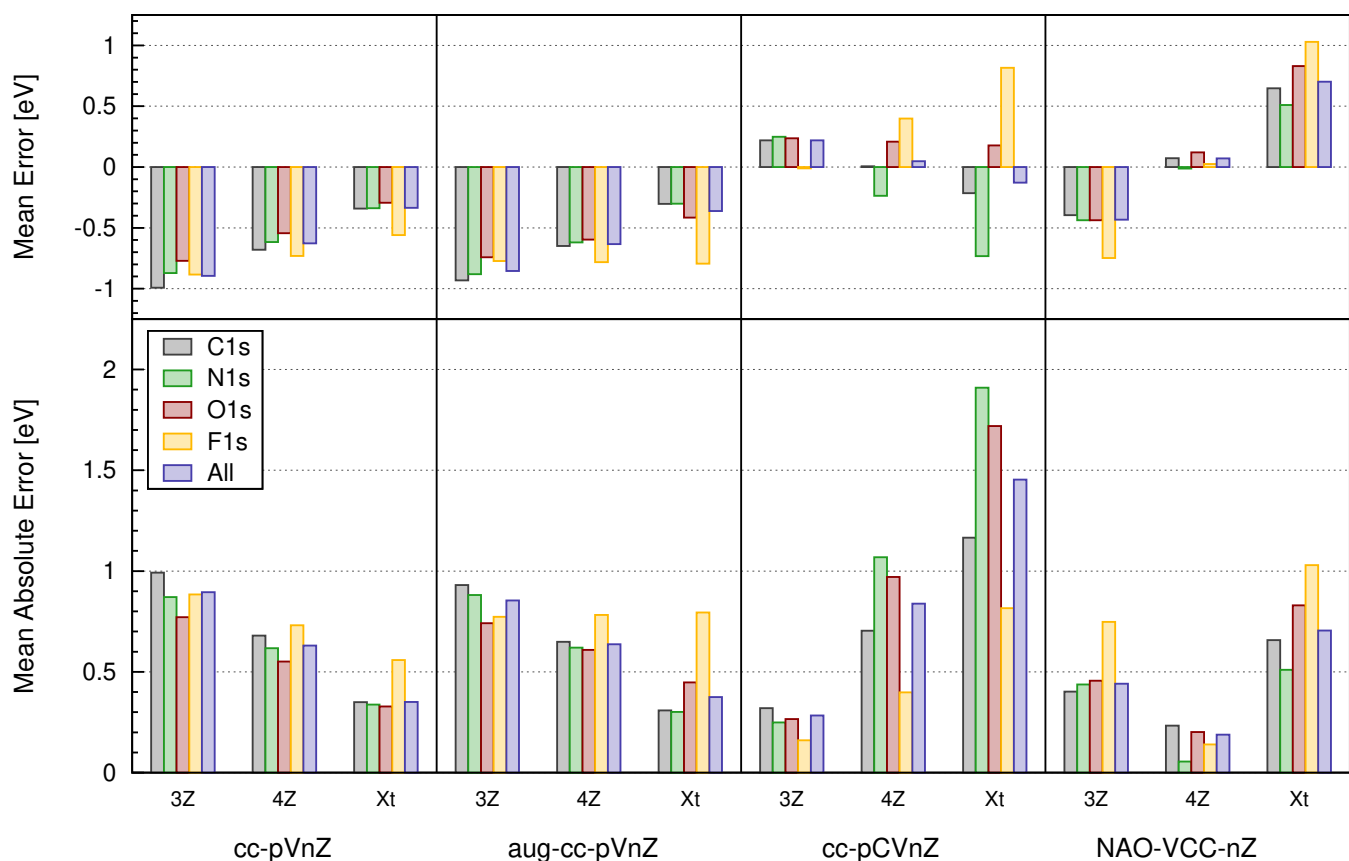

**Figure S1:** Mean error (above) and absolute mean error (below) for the computed non-relativistic 65  $\text{evGW}_0\text{@PBE+RC}$  1s binding energies calculated at the 3Z and 4Z level in the labeled basis set series. Extrapolated values (Xt) are calculated with a 2 point linear extrapolation against the inverse of the number of basis functions. The error in the computed binding energy is defined as  $\text{Error}_i = \text{BE}_i^{\text{theory}} - \text{BE}_i^{\text{exp}}$ .

## 4 Core-level binding energies with aZORA

**Table S3:** Core-level binding energies (BEs) from  $\text{evGW}_0\text{@PBE+aZORA}$  using the cc-pVnZ basis set series with  $n = 3 - 6$ . Extrapolated values ( $\infty$ ), standard error (SE) and correlation coefficient  $R^2$ . The last column indicates the basis sets used for the extrapolation; for most cases all data points ( $n = 3 - 6$ ) are included. All values in eV.

| CAS      | name               | formula                | core level | $\text{evGW}_0\text{@PBE+aZORA}$ |         |         |         |          | SE   | $R^2$ | $n$ used |
|----------|--------------------|------------------------|------------|----------------------------------|---------|---------|---------|----------|------|-------|----------|
|          |                    |                        |            | $n = 3$                          | $n = 4$ | $n = 5$ | $n = 6$ | $\infty$ |      |       |          |
| 74-82-8  | methane            | $\text{CH}_4$          | C1s        | 290.07                           | 290.32  | 290.45  | 290.75  | 290.74   | 0.12 | 0.86  | 3-6      |
| 74-84-0  | ethane             | $\text{C}_2\text{H}_6$ | C1s        | 289.97                           | 290.24  | 290.39  | 290.67  | 290.69   | 0.10 | 0.90  | 3-6      |
| 74-85-1  | ethene             | $\text{C}_2\text{H}_4$ | C1s        | 290.26                           | 290.52  | 290.63  | 290.83  | 290.87   | 0.07 | 0.94  | 3-6      |
| 74-86-2  | ethyne             | $\text{C}_2\text{H}_2$ | C1s        | 290.77                           | 291.01  | 291.05  | 291.23  | 291.27   | 0.06 | 0.93  | 3-6      |
| 630-08-0 | carbon monoxide    | CO                     | O1s        | 542.12                           | 542.33  | 542.39  | 542.49  | 542.56   | 0.02 | 0.98  | 3-6      |
| 630-08-0 | carbon monoxide    | CO                     | C1s        | 295.35                           | 295.62  | 295.65  | 295.78  | 295.87   | 0.04 | 0.97  | 3-6      |
| 124-38-9 | carbon dioxide     | $\text{CO}_2$          | O1s        | 540.89                           | 541.07  | 541.08  | 541.23  | 541.26   | 0.05 | 0.91  | 3-6      |
| 124-38-9 | carbon dioxide     | $\text{CO}_2$          | C1s        | 296.38                           | 296.70  | 296.82  | 297.05  | 297.15   | 0.07 | 0.95  | 3-6      |
| 75-73-0  | tetrafluoromethane | $\text{CF}_4$          | F1s        | 694.79                           | 694.84  | 694.93  | 695.07  | 695.18   | 0.08 | 0.91  | 4-6      |
| 75-73-0  | tetrafluoromethane | $\text{CF}_4$          | C1s        | 300.12                           | 300.53  | 300.68  | 300.91  | 301.05   | 0.06 | 0.98  | 3-6      |
| 593-53-3 | fluoromethane      | $\text{CH}_3\text{F}$  | F1s        | 692.40                           | 692.51  | 692.44  | 692.59  | 692.63   | 0.00 | 1.00  | 3,4,6    |
| 593-53-3 | fluoromethane      | $\text{CH}_3\text{F}$  | C1s        | 292.69                           | 293.02  | 293.18  | 293.39  | 293.46   | 0.07 | 0.96  | 3-6      |

Table S3: Continued

| CAS        | name             | formula                                       | core level              | evGW <sub>0</sub> @PBE+aZORA |        |        |        |        | SE   | R <sup>2</sup> | n used |
|------------|------------------|-----------------------------------------------|-------------------------|------------------------------|--------|--------|--------|--------|------|----------------|--------|
|            |                  |                                               |                         | n = 3                        | n = 4  | n = 5  | n = 6  | ∞      |      |                |        |
| 75-46-7    | trifluoromethane | CHF <sub>3</sub>                              | F1s                     | 694.00                       | 694.07 | 694.10 | 694.25 | 694.14 | 0.00 | 1.00           | 3-5    |
| 75-46-7    | trifluoromethane | CHF <sub>3</sub>                              | C1s                     | 297.74                       | 298.15 | 298.31 | 298.51 | 298.65 | 0.05 | 0.98           | 3-6    |
| 67-56-1    | methanol         | CH <sub>3</sub> OH                            | O1s                     | 538.70                       | 538.81 | 538.79 | 538.94 | 538.98 | 0.03 | 0.97           | 3,4,6  |
| 67-56-1    | methanol         | CH <sub>3</sub> OH                            | C1s                     | 291.65                       | 291.97 | 292.08 | 292.40 | 292.42 | 0.11 | 0.90           | 3-6    |
| 50-00-0    | formaldehyde     | CH <sub>2</sub> O                             | O1s                     | 539.00                       | 539.28 | 539.28 | 539.39 | 539.46 | 0.05 | 0.94           | 3-6    |
| 50-00-0    | formaldehyde     | CH <sub>2</sub> O                             | C1s                     | 293.72                       | 294.12 | 294.21 | 294.39 | 294.50 | 0.05 | 0.98           | 3-6    |
| 115-10-6   | dimethyl ether   | CH <sub>3</sub> OCH <sub>3</sub>              | O1s                     | 538.26                       | 538.33 | 538.37 | 538.52 | 538.41 | 0.01 | 0.99           | 3-5    |
| 115-10-6   | dimethyl ether   | CH <sub>3</sub> OCH <sub>3</sub>              | C1s                     | 291.45                       | 291.76 | 297.98 | 292.17 | 292.27 | 0.11 | 0.96           | 3,4,6  |
| 64-18-6    | formic acid      | HCOOH                                         | O1s (OH)                | 540.23                       | 540.37 | 540.37 | 540.53 | 540.59 | 0.03 | 0.98           | 3,4,6  |
| 64-18-6    | formic acid      | HCOOH                                         | O1s (C=O)               | 538.33                       | 538.61 | 538.60 | 538.72 | 538.79 | 0.06 | 0.92           | 3-6    |
| 64-18-6    | formic acid      | HCOOH                                         | C1s                     | 294.59                       | 295.00 | 295.07 | 295.31 | 295.41 | 0.07 | 0.96           | 3-6    |
| 67-64-1    | acetone          | (CH <sub>3</sub> ) <sub>2</sub> CO            | O1s                     | 537.41                       | 537.60 | 537.61 | 537.75 | 537.77 | 0.05 | 0.90           | 3-6    |
| 67-64-1    | acetone          | (CH <sub>3</sub> ) <sub>2</sub> CO            | C1s (C=O)               | 292.80                       | 293.08 | 293.25 | 293.41 | 293.49 | 0.05 | 0.97           | 3-6    |
| 67-64-1    | acetone          | (CH <sub>3</sub> ) <sub>2</sub> CO            | C1s (CH <sub>3</sub> )  | 290.36                       | 290.64 | 290.83 | 291.03 | 291.10 | 0.07 | 0.95           | 3-6    |
| 107-31-3   | methyl formate   | HCO <sub>2</sub> CH <sub>3</sub>              | O1s (OCH <sub>3</sub> ) | 539.58                       | 539.65 | 539.72 | 539.94 | 539.77 | 0.03 | 0.95           | 3-5    |
| 107-31-3   | methyl formate   | HCO <sub>2</sub> CH <sub>3</sub>              | O1s (C=O)               | 537.87                       | 538.17 | 538.14 | 538.26 | 538.33 | 0.06 | 0.91           | 3-6    |
| 64-19-7    | acetic acid      | CH <sub>3</sub> COOH                          | O1s (OH)                | 539.57                       | 539.78 | 539.77 | 539.94 | 539.96 | 0.06 | 0.88           | 3-6    |
| 64-19-7    | acetic acid      | CH <sub>3</sub> COOH                          | O1s (C=O)               | 537.64                       | 537.89 | 537.88 | 538.01 | 538.06 | 0.05 | 0.92           | 3-6    |
| 64-19-7    | acetic acid      | CH <sub>3</sub> COOH                          | C1s (COOH)              | 294.22                       | 294.48 | 294.62 | 294.90 | 294.93 | 0.11 | 0.90           | 3-6    |
| 64-19-7    | acetic acid      | CH <sub>3</sub> COOH                          | C1s (CH <sub>3</sub> )  | 290.79                       | 291.02 | 291.18 | 291.49 | 291.51 | 0.13 | 0.86           | 3-6    |
| 7732-18-5  | water            | H <sub>2</sub> O                              | O1s                     | 539.46                       | 539.56 | 539.50 | 539.61 | 539.65 | 0.01 | 0.99           | 3,4,6  |
| 10028-15-6 | ozone            | O <sub>3</sub>                                | O1s middle              | 546.74                       | 546.89 | 546.98 | 547.12 | 547.16 | 0.05 | 0.92           | 3-6    |
| 10028-15-6 | ozone            | O <sub>3</sub>                                | O1s terminal            | 541.43                       | 541.56 | 541.60 | 541.68 | 541.72 | 0.02 | 0.97           | 3-6    |
| 7782-44-7  | oxygen           | O <sub>2</sub>                                | O1s weaker              | 544.09                       | 544.32 | 544.25 | 544.32 | 544.36 | 0.03 | 0.98           | 3,5,6  |
| 7782-44-7  | oxygen           | O <sub>2</sub>                                | O1s stronger            | 542.84                       | 543.13 | 543.19 | 543.26 | 543.38 | 0.03 | 0.98           | 3-6    |
| 7727-37-9  | nitrogen         | N <sub>2</sub>                                | N1s                     | 409.18                       | 409.54 | 409.66 | 409.82 | 409.96 | 0.04 | 0.99           | 3-6    |
| 7664-41-7  | ammonia          | NH <sub>3</sub>                               | N1s                     | 405.10                       | 405.19 | 405.26 | 405.52 | 405.31 | 0.02 | 0.98           | 3-5    |
| 74-90-8    | hydrogen cyanide | HCN                                           | N1s                     | 406.22                       | 406.57 | 406.55 | 406.85 | 406.89 | 0.11 | 0.86           | 3-6    |
| 74-90-8    | hydrogen cyanide | HCN                                           | C1s                     | 292.74                       | 293.02 | 293.06 | 293.26 | 293.31 | 0.07 | 0.92           | 3-6    |
| 75-05-8    | acetonitrile     | CH <sub>3</sub> CN                            | N1s                     | 404.96                       | 405.28 | 405.27 | 405.56 | 405.59 | 0.10 | 0.87           | 3-6    |
| 75-05-8    | acetonitrile     | CH <sub>3</sub> CN                            | C1s (CH <sub>3</sub> )  | 291.90                       | 292.18 | 292.29 | 292.55 | 292.59 | 0.09 | 0.91           | 3-6    |
| 75-05-8    | acetonitrile     | CH <sub>3</sub> CN                            | C1s (CN)                | 291.94                       | 292.17 | 292.26 | 292.47 | 292.51 | 0.07 | 0.92           | 3-6    |
| 56-40-6    | glycine          | C <sub>2</sub> H <sub>5</sub> NO <sub>2</sub> | O1s (OH)                | 539.65                       | 539.76 | 539.81 | 540.06 | 539.88 | 0.00 | 1.00           | 3-5    |
| 56-40-6    | glycine          | C <sub>2</sub> H <sub>5</sub> NO <sub>2</sub> | O1s (C=O)               | 537.73                       | 537.94 | 537.97 | 538.11 | 538.15 | 0.05 | 0.94           | 3-6    |
| 56-40-6    | glycine          | C <sub>2</sub> H <sub>5</sub> NO <sub>2</sub> | N1s                     | 404.97                       | 405.10 | 405.16 | 405.46 | 405.25 | 0.00 | 1.00           | 3-5    |
| 56-40-6    | glycine          | C <sub>2</sub> H <sub>5</sub> NO <sub>2</sub> | C1s (COOH)              | 293.94                       | 294.34 | 294.42 | 294.70 | 294.78 | 0.09 | 0.94           | 3-6    |
| 56-40-6    | glycine          | C <sub>2</sub> H <sub>5</sub> NO <sub>2</sub> | C1s (CH <sub>2</sub> )  | 291.36                       | 291.75 | 291.86 | 292.16 | 292.23 | 0.09 | 0.94           | 3-6    |
| 110-86-1   | pyridine         | C <sub>5</sub> H <sub>5</sub> N               | N1s                     | 404.16                       | 404.37 | 404.48 | 404.70 | 404.73 | 0.08 | 0.90           | 3-6    |
| 109-97-7   | pyrrole          | C <sub>4</sub> H <sub>4</sub> NH              | N1s                     | 405.50                       | 405.73 | 405.92 | 406.13 | 406.18 | 0.08 | 0.93           | 3-6    |
| 62-53-3    | aniline          | C <sub>6</sub> H <sub>5</sub> NH <sub>2</sub> | N1s                     | 404.51                       | 404.80 | 404.90 | 405.24 | 405.26 | 0.13 | 0.87           | 3-6    |
| 57-13-6    | urea             | CO(NH <sub>2</sub> ) <sub>2</sub>             | O1s                     | 536.49                       | 536.72 | 536.76 | 536.87 | 536.93 | 0.03 | 0.97           | 3-6    |
| 57-13-6    | urea             | CO(NH <sub>2</sub> ) <sub>2</sub>             | N1s                     | 405.44                       | 405.61 | 405.76 | 406.00 | 406.01 | 0.11 | 0.85           | 3-6    |
| 57-13-6    | urea             | CO(NH <sub>2</sub> ) <sub>2</sub>             | C1s                     | 293.69                       | 293.99 | 294.19 | 294.43 | 294.50 | 0.09 | 0.94           | 3-6    |
| 74-89-5    | methylamine      | CH <sub>3</sub> NH <sub>2</sub>               | N1s                     | 404.74                       | 404.88 | 404.91 | 405.20 | 404.99 | 0.02 | 0.99           | 3-5    |
| 98-95-3    | nitrobenzene     | C <sub>6</sub> H <sub>5</sub> NO <sub>2</sub> | O1s                     | 538.06                       | 538.30 | 538.40 | 538.47 | 538.56 | 0.00 | 1.00           | 3-6    |
| 98-95-3    | nitrobenzene     | C <sub>6</sub> H <sub>5</sub> NO <sub>2</sub> | N1s                     | 410.72                       | 410.97 | 411.19 | 411.32 | 411.42 | 0.06 | 0.97           | 3-6    |
| 98-95-3    | nitrobenzene     | C <sub>6</sub> H <sub>5</sub> NO <sub>2</sub> | C1s (C1)                | 291.23                       | 291.52 | 291.76 | 291.88 | 292.01 | 0.05 | 0.98           | 3-6    |
| 98-95-3    | nitrobenzene     | C <sub>6</sub> H <sub>5</sub> NO <sub>2</sub> | C1s (C2-4)              | 290.33                       | 290.63 | 290.85 | 292.67 | 291.06 | 0.06 | 0.99           | 3-5    |
| 71-43-2    | benzene          | C <sub>6</sub> H <sub>6</sub>                 | C1s                     | 289.66                       | 289.93 | 290.05 | 290.28 | 290.33 | 0.07 | 0.94           | 3-6    |
| 536-74-3   | phenylacetylene  | C <sub>8</sub> H <sub>6</sub>                 | C1s (C3)                | 290.28                       | 290.56 | 290.72 | 290.94 | 291.00 | 0.07 | 0.95           | 3-6    |

Table S3: Continued

| CAS      | name            | formula                       | core level | evGW <sub>0</sub> @PBE+aZORA |        |        |        |        | SE   | R <sup>2</sup> | n used |
|----------|-----------------|-------------------------------|------------|------------------------------|--------|--------|--------|--------|------|----------------|--------|
|          |                 |                               |            | n = 3                        | n = 4  | n = 5  | n = 6  | ∞      |      |                |        |
| 536-74-3 | phenylacetylene | C <sub>8</sub> H <sub>6</sub> | C1s (C2)   | 289.84                       | 290.16 | 290.27 | 290.49 | 290.56 | 0.07 | 0.95           | 3-6    |
| 536-74-3 | phenylacetylene | C <sub>8</sub> H <sub>6</sub> | C1s (C4-6) | 289.65                       | 289.96 | 290.10 | 290.30 | 290.38 | 0.06 | 0.96           | 3-6    |
| 536-74-3 | phenylacetylene | C <sub>8</sub> H <sub>6</sub> | C1s (C1)   | 289.37                       | 289.63 | 289.71 | 289.95 | 289.99 | 0.08 | 0.91           | 3-6    |

**Table S4:** Core-level binding energies (BEs) as obtained from evGW<sub>0</sub>@PBE+aZORA and evGW<sub>0</sub>@PBE+aZORA+RC and their deviation from experiment  $\Delta_{\text{exp},i} = \text{BE}_i^{\text{theory}} - \text{BE}_i^{\text{exp}}$ . All values in eV. The BEs from GW have been extrapolated to the complete basis set limit by performing a linear regression with respect to the inverse of the total number of basis functions using the cc-pVnZ basis set series ( $n = 3 - 6$ ). Corresponding results for non-relativistic evGW<sub>0</sub> and evGW<sub>0</sub>+RC are given in the supplement to Ref. 14.

| name               | formula                            | core level              | evGW <sub>0</sub> @PBE+aZORA |                       | evGW <sub>0</sub> @PBE+aZORA+RC |                       | Exp.   | Ref <sub>Exp.</sub> |
|--------------------|------------------------------------|-------------------------|------------------------------|-----------------------|---------------------------------|-----------------------|--------|---------------------|
|                    |                                    |                         | BE                           | $\Delta_{\text{exp}}$ | BE                              | $\Delta_{\text{exp}}$ |        |                     |
| methane            | CH <sub>4</sub>                    | C1s                     | 290.74                       | -0.10                 | 290.64                          | -0.20                 | 290.84 | 15                  |
| ethane             | C <sub>2</sub> H <sub>6</sub>      | C1s                     | 290.69                       | -0.03                 | 290.59                          | -0.13                 | 290.71 | 15                  |
| ethene             | C <sub>2</sub> H <sub>4</sub>      | C1s                     | 290.87                       | 0.05                  | 290.77                          | -0.05                 | 290.82 | 15                  |
| ethyne             | C <sub>2</sub> H <sub>2</sub>      | C1s                     | 291.27                       | 0.03                  | 291.17                          | -0.07                 | 291.25 | 15                  |
| carbon monoxide    | CO                                 | O1s                     | 542.56                       | 0.46                  | 542.20                          | 0.10                  | 542.1  | 16                  |
| carbon monoxide    | CO                                 | C1s                     | 295.87                       | -0.36                 | 295.77                          | -0.46                 | 296.23 | 15                  |
| carbon dioxide     | CO <sub>2</sub>                    | O1s                     | 541.26                       | -0.06                 | 540.90                          | -0.42                 | 541.32 | 17                  |
| carbon dioxide     | CO <sub>2</sub>                    | C1s                     | 297.15                       | -0.55                 | 297.05                          | -0.65                 | 297.70 | 15                  |
| tetrafluoromethane | CF <sub>4</sub>                    | F1s                     | 695.18                       | -0.02                 | 694.58                          | -0.62                 | 695.2  | 16                  |
| tetrafluoromethane | CF <sub>4</sub>                    | C1s                     | 301.05                       | -0.85                 | 300.95                          | -0.95                 | 301.90 | 15                  |
| fluoromethane      | CH <sub>3</sub> F                  | F1s                     | 692.63                       | 0.23                  | 692.03                          | -0.37                 | 692.4  | 18                  |
| fluoromethane      | CH <sub>3</sub> F                  | C1s                     | 293.46                       | -0.09                 | 293.36                          | -0.19                 | 293.56 | 15                  |
| trifluoromethane   | CHF <sub>3</sub>                   | F1s                     | 694.14                       | 0.04                  | 693.54                          | -0.56                 | 694.1  | 18                  |
| trifluoromethane   | CHF <sub>3</sub>                   | C1s                     | 298.65                       | -0.51                 | 298.55                          | -0.61                 | 299.16 | 15                  |
| methanol           | CH <sub>3</sub> OH                 | O1s                     | 538.98                       | 0.10                  | 538.62                          | -0.26                 | 538.88 | 19 (16,20)          |
| methanol           | CH <sub>3</sub> OH                 | C1s                     | 292.42                       | 0.12                  | 292.32                          | 0.02                  | 292.30 | 16,19               |
| formaldehyde       | CH <sub>2</sub> O                  | O1s                     | 539.46                       | 0.13                  | 539.10                          | -0.23                 | 539.33 | 19 (16,20)          |
| formaldehyde       | CH <sub>2</sub> O                  | C1s                     | 294.50                       | 0.12                  | 294.40                          | 0.02                  | 294.38 | 19                  |
| dimethyl ether     | CH <sub>3</sub> OCH <sub>3</sub>   | O1s                     | 538.41                       | 0.05                  | 538.05                          | -0.31                 | 538.36 | 19 (16,20)          |
| dimethyl ether     | CH <sub>3</sub> OCH <sub>3</sub>   | C1s                     | 292.27                       | 0.10                  | 292.17                          | 0.00                  | 292.17 | 21                  |
| formic acid        | HCOOH                              | O1s (OH)                | 540.59                       | -0.10                 | 540.23                          | -0.46                 | 540.69 | 22                  |
| formic acid        | HCOOH                              | O1s (C=O)               | 538.79                       | -0.23                 | 538.43                          | -0.59                 | 539.02 | 22                  |
| formic acid        | HCOOH                              | C1s                     | 295.41                       | -0.34                 | 295.31                          | -0.44                 | 295.75 | 22                  |
| acetone            | (CH <sub>3</sub> ) <sub>2</sub> CO | O1s                     | 537.77                       | 0.04                  | 537.42                          | -0.31                 | 537.73 | 19 (16,20)          |
| acetone            | (CH <sub>3</sub> ) <sub>2</sub> CO | C1s (C=O)               | 293.49                       | -0.39                 | 293.39                          | -0.49                 | 293.88 | 19                  |
| acetone            | (CH <sub>3</sub> ) <sub>2</sub> CO | C1s (CH <sub>3</sub> )  | 291.10                       | -0.13                 | 291.00                          | -0.23                 | 291.23 | 19                  |
| methyl formate     | HCO <sub>2</sub> CH <sub>3</sub>   | O1s (OCH <sub>3</sub> ) | 539.77                       | 0.13                  | 539.41                          | -0.23                 | 539.64 | 19 (16,20)          |
| methyl formate     | HCO <sub>2</sub> CH <sub>3</sub>   | O1s (C=O)               | 538.33                       | 0.09                  | 537.97                          | -0.27                 | 538.24 | 19 (16,20)          |
| acetic acid        | CH <sub>3</sub> COOH               | O1s (OH)                | 539.96                       | -0.14                 | 539.60                          | -0.50                 | 540.10 | 22                  |
| acetic acid        | CH <sub>3</sub> COOH               | O1s (C=O)               | 538.06                       | -0.25                 | 537.70                          | -0.61                 | 538.31 | 22                  |
| acetic acid        | CH <sub>3</sub> COOH               | C1s (COOH)              | 294.93                       | -0.42                 | 294.83                          | -0.52                 | 295.35 | 22                  |
| acetic acid        | CH <sub>3</sub> COOH               | C1s (CH <sub>3</sub> )  | 291.51                       | -0.04                 | 291.41                          | -0.14                 | 291.55 | 22                  |
| water              | H <sub>2</sub> O                   | O1s                     | 539.65                       | -0.05                 | 539.29                          | -0.41                 | 539.7  | 16                  |
| ozone              | O <sub>3</sub>                     | O1s middle              | 547.16                       | 0.72                  | 546.80                          | 0.36                  | 546.44 | 23                  |
| ozone              | O <sub>3</sub>                     | O1s terminal            | 541.72                       | -0.03                 | 541.36                          | -0.39                 | 541.75 | 23                  |
| oxygen             | O <sub>2</sub>                     | O1s weaker              | 544.36                       | 0.16                  | 544.00                          | -0.20                 | 544.2  | 16                  |
| oxygen             | O <sub>2</sub>                     | O1s stronger            | 543.38                       | 0.28                  | 543.02                          | -0.08                 | 543.1  | 16                  |

**Table S4:** Continued

| name             | formula                                       | core level             | evGW <sub>0</sub> @PBE+aZORA |                       | evGW <sub>0</sub> @PBE+aZORA+RC |                       | Exp.   | Ref <sub>Exp.</sub> |
|------------------|-----------------------------------------------|------------------------|------------------------------|-----------------------|---------------------------------|-----------------------|--------|---------------------|
|                  |                                               |                        | BE                           | $\Delta_{\text{exp}}$ | BE                              | $\Delta_{\text{exp}}$ |        |                     |
| nitrogen         | N <sub>2</sub>                                | N1s                    | 409.96                       | 0.03                  | 409.76                          | -0.17                 | 409.93 | 17                  |
| ammonia          | NH <sub>3</sub>                               | N1s                    | 405.31                       | -0.21                 | 405.11                          | -0.41                 | 405.52 | 19(17,20)           |
| hydrogen cyanide | HCN                                           | N1s                    | 406.89                       | 0.09                  | 406.69                          | -0.11                 | 406.8  | 19 (17,24)          |
| hydrogen cyanide | HCN                                           | C1s                    | 293.31                       | -0.19                 | 293.21                          | -0.29                 | 293.5  | 19                  |
| acetonitrile     | CH <sub>3</sub> CN                            | N1s                    | 405.59                       | 0.01                  | 405.39                          | -0.19                 | 405.58 | 25                  |
| acetonitrile     | CH <sub>3</sub> CN                            | C1s (CH <sub>3</sub> ) | 292.59                       | -0.29                 | 292.49                          | -0.39                 | 292.88 | 25                  |
| acetonitrile     | CH <sub>3</sub> CN                            | C1s (CN)               | 292.51                       | -0.09                 | 292.41                          | -0.19                 | 292.60 | 25                  |
| glycine          | C <sub>2</sub> H <sub>5</sub> NO <sub>2</sub> | O1s (OH)               | 539.88                       | -0.32                 | 539.52                          | -0.68                 | 540.2  | 26                  |
| glycine          | C <sub>2</sub> H <sub>5</sub> NO <sub>2</sub> | O1s (C=O)              | 538.15                       | -0.25                 | 537.79                          | -0.61                 | 538.4  | 26                  |
| glycine          | C <sub>2</sub> H <sub>5</sub> NO <sub>2</sub> | N1s                    | 405.25                       | -0.15                 | 405.05                          | -0.35                 | 405.4  | 26                  |
| glycine          | C <sub>2</sub> H <sub>5</sub> NO <sub>2</sub> | C1s (COOH)             | 294.78                       | -0.42                 | 294.68                          | -0.52                 | 295.2  | 26                  |
| glycine          | C <sub>2</sub> H <sub>5</sub> NO <sub>2</sub> | C1s (CH <sub>2</sub> ) | 292.23                       | -0.07                 | 292.13                          | -0.17                 | 292.3  | 26                  |
| pyridine         | C <sub>5</sub> H <sub>5</sub> N               | N1s                    | 404.73                       | -0.09                 | 404.53                          | -0.29                 | 404.82 | 27                  |
| pyrrole          | C <sub>4</sub> H <sub>4</sub> NH              | N1s                    | 406.18                       | -0.00                 | 405.98                          | -0.20                 | 406.18 | 27                  |
| aniline          | C <sub>6</sub> H <sub>5</sub> NH <sub>2</sub> | N1s                    | 405.26                       | -0.05                 | 405.06                          | -0.25                 | 405.31 | 27                  |
| urea             | CO(NH <sub>2</sub> ) <sub>2</sub>             | O1s                    | 536.93                       | -0.26                 | 536.57                          | -0.62                 | 537.19 | 19                  |
| urea             | CO(NH <sub>2</sub> ) <sub>2</sub>             | N1s                    | 406.01                       | -0.08                 | 405.82                          | -0.27                 | 406.09 | 19                  |
| urea             | CO(NH <sub>2</sub> ) <sub>2</sub>             | C1s                    | 294.50                       | -0.34                 | 294.40                          | -0.44                 | 294.84 | 19                  |
| methylamine      | CH <sub>3</sub> NH <sub>2</sub>               | N1s                    | 404.99                       | -0.18                 | 404.79                          | -0.38                 | 405.17 | 19 (17,20)          |
| nitrobenzene     | C <sub>6</sub> H <sub>5</sub> NO <sub>2</sub> | O1s                    | 538.56                       | -0.07                 | 538.21                          | -0.42                 | 538.63 | 19                  |
| nitrobenzene     | C <sub>6</sub> H <sub>5</sub> NO <sub>2</sub> | N1s                    | 411.42                       | -0.18                 | 411.22                          | -0.38                 | 411.6  | 16                  |
| nitrobenzene     | C <sub>6</sub> H <sub>5</sub> NO <sub>2</sub> | C1s (C1)               | 292.01                       | -0.07                 | 291.91                          | -0.17                 | 292.08 | 19                  |
| nitrobenzene     | C <sub>6</sub> H <sub>5</sub> NO <sub>2</sub> | C1s (C2-4)             | 291.06                       | -0.07                 | 290.96                          | -0.17                 | 291.13 | 19                  |
| benzene          | C <sub>6</sub> H <sub>6</sub>                 | C1s                    | 290.33                       | -0.05                 | 290.23                          | -0.15                 | 290.38 | 28                  |
| phenylacetylene  | C <sub>8</sub> H <sub>6</sub>                 | C1s (C3)               | 291.00                       | 0.12                  | 290.90                          | 0.02                  | 290.88 | 29                  |
| phenylacetylene  | C <sub>8</sub> H <sub>6</sub>                 | C1s (C2)               | 290.56                       | 0.01                  | 290.46                          | -0.09                 | 290.55 | 29                  |
| phenylacetylene  | C <sub>8</sub> H <sub>6</sub>                 | C1s (C4-6)             | 290.38                       | 0.22                  | 290.28                          | 0.12                  | 290.16 | 29                  |
| phenylacetylene  | C <sub>8</sub> H <sub>6</sub>                 | C1s (C1)               | 289.99                       | 0.24                  | 289.89                          | 0.14                  | 289.75 | 29                  |

## 5 Non-relativistic $\Delta$ SCF and pre-corrected evGW<sub>0</sub> results

**Table S5:** Core-level binding energies (BEs) as obtained from non-relativistic  $\Delta$ SCF, evGW<sub>0</sub>@PBE with shifted eigenvalues (applying atomic corrections  $\Delta\epsilon_{\text{1s,at}}^{\text{SKS}}$  to DFT eigenvalues, pre-correction), and deviation from experiment  $\Delta_{\text{exp},i} = \text{BE}_i^{\text{theory}} - \text{BE}_i^{\text{exp}}$ . All values in eV. The  $\Delta$ SCF values have been computed at the PBE0 level employing uncontracted def2-QZVP basis sets. The pre-corrected evGW<sub>0</sub> values (evGW<sub>0</sub>@PBE(pre)) have been extrapolated against the inverse of the number of basis functions using the cc-pVnZ (n=3,4) basis sets. Corresponding results for  $\Delta$ SCF with aZORA are given in the supplement to Ref. 14.

| name               | formula                       | core level | $\Delta$ SCF |                       | evGW <sub>0</sub> @PBE(pre) |                       | BE     | Ref <sub>Exp.</sub> |
|--------------------|-------------------------------|------------|--------------|-----------------------|-----------------------------|-----------------------|--------|---------------------|
|                    |                               |            | BE           | $\Delta_{\text{exp}}$ | BE                          | $\Delta_{\text{exp}}$ |        |                     |
| methane            | CH <sub>4</sub>               | C1s        | 290.21       | -0.63                 | 290.44                      | -0.40                 | 290.84 | 15                  |
| ethane             | C <sub>2</sub> H <sub>6</sub> | C1s        | 290.08       | -0.63                 | 290.46                      | -0.25                 | 290.71 | 15                  |
| ethene             | C <sub>2</sub> H <sub>4</sub> | C1s        | 290.18       | -0.64                 | 290.68                      | -0.14                 | 290.82 | 15                  |
| ethyne             | C <sub>2</sub> H <sub>2</sub> | C1s        | 290.74       | -0.51                 | 291.11                      | -0.14                 | 291.25 | 15                  |
| carbon monoxide    | CO                            | O1s        | 541.37       | -0.73                 | 542.09                      | -0.01                 | 542.1  | 16                  |
| carbon monoxide    | CO                            | C1s        | 295.84       | -0.39                 | 295.86                      | -0.37                 | 296.23 | 15                  |
| carbon dioxide     | CO <sub>2</sub>               | O1s        | 540.20       | -1.12                 | 540.89                      | -0.43                 | 541.32 | 17                  |
| carbon dioxide     | CO <sub>2</sub>               | C1s        | 297.18       | -0.52                 | 297.00                      | -0.70                 | 297.70 | 15                  |
| tetrafluoromethane | CF <sub>4</sub>               | F1s        | 693.68       | -1.52                 | 694.37                      | -0.83                 | 695.2  | 16                  |

Table S5: Continued

| name               | formula                                       | core level              | $\Delta$ SCF |                       | evGW <sub>0</sub> @PBE(pre) |                       | BE     | Ref <sub>Exp.</sub> |
|--------------------|-----------------------------------------------|-------------------------|--------------|-----------------------|-----------------------------|-----------------------|--------|---------------------|
|                    |                                               |                         | BE           | $\Delta_{\text{exp}}$ | BE                          | $\Delta_{\text{exp}}$ |        |                     |
| tetrafluoromethane | CF <sub>4</sub>                               | C1s                     | 301.03       | -0.86                 | 300.94                      | -0.96                 | 301.90 | 15                  |
| fluoromethane      | CH <sub>3</sub> F                             | F1s                     | 691.10       | -1.30                 | 692.05                      | -0.35                 | 692.4  | 18                  |
| fluoromethane      | CH <sub>3</sub> F                             | C1s                     | 292.92       | -0.64                 | 293.26                      | -0.30                 | 293.56 | 15                  |
| trifluoromethane   | CHF <sub>3</sub>                              | F1s                     | 692.84       | -1.26                 | 693.58                      | -0.52                 | 694.1  | 18                  |
| trifluoromethane   | CHF <sub>3</sub>                              | C1s                     | 298.39       | -0.77                 | 298.54                      | -0.62                 | 299.16 | 15                  |
| methanol           | CH <sub>3</sub> OH                            | O1s                     | 537.89       | -0.99                 | 538.59                      | -0.29                 | 538.88 | 19 (16,20)          |
| methanol           | CH <sub>3</sub> OH                            | C1s                     | 291.82       | -0.48                 | 292.19                      | -0.11                 | 292.30 | 16,19               |
| formaldehyde       | CH <sub>2</sub> O                             | O1s                     | 538.20       | -1.13                 | 539.22                      | -0.11                 | 539.33 | 19 (16,20)          |
| formaldehyde       | CH <sub>2</sub> O                             | C1s                     | 293.92       | -0.46                 | 294.45                      | 0.07                  | 294.38 | 19                  |
| dimethyl ether     | CH <sub>3</sub> OCH <sub>3</sub>              | O1s                     | 537.41       | -0.95                 | 538.06                      | -0.30                 | 538.36 | 19 (16,20)          |
| dimethyl ether     | CH <sub>3</sub> OCH <sub>3</sub>              | C1s                     | 291.57       | -0.60                 | 291.97                      | -0.20                 | 292.17 | 21                  |
| formic acid        | HCOOH                                         | O1s (OH)                | 539.55       | -1.14                 | 540.20                      | -0.49                 | 540.69 | 22                  |
| formic acid        | HCOOH                                         | O1s (C=O)               | 537.67       | -1.35                 | 538.59                      | -0.43                 | 539.02 | 22                  |
| formic acid        | HCOOH                                         | C1s                     | 295.13       | -0.62                 | 295.38                      | -0.37                 | 295.75 | 22                  |
| acetone            | (CH <sub>3</sub> ) <sub>2</sub> CO            | O1s                     | 536.59       | -1.14                 | 537.45                      | -0.28                 | 537.73 | 19 (16,20)          |
| acetone            | (CH <sub>3</sub> ) <sub>2</sub> CO            | C1s (C=O)               | 293.07       | -0.81                 | 293.27                      | -0.61                 | 293.88 | 19                  |
| acetone            | (CH <sub>3</sub> ) <sub>2</sub> CO            | C1s (CH <sub>3</sub> )  | 290.53       | -0.70                 | 290.83                      | -0.40                 | 291.23 | 19                  |
| methyl formate     | HCO <sub>2</sub> CH <sub>3</sub>              | O1s (OCH <sub>3</sub> ) | 538.76       | -0.88                 | 539.46                      | -0.18                 | 539.64 | 19 (16,20)          |
| methyl formate     | HCO <sub>2</sub> CH <sub>3</sub>              | O1s (C=O)               | 537.19       | -1.05                 | 538.14                      | -0.10                 | 538.24 | 19 (16,20)          |
| acetic acid        | CH <sub>3</sub> COOH                          | O1s (OH)                | 538.98       | -1.12                 | 539.58                      | -0.52                 | 540.10 | 22                  |
| acetic acid        | CH <sub>3</sub> COOH                          | O1s (C=O)               | 536.96       | -1.35                 | 537.81                      | -0.50                 | 538.31 | 22                  |
| acetic acid        | CH <sub>3</sub> COOH                          | C1s (COOH)              | 294.70       | -0.65                 | 294.68                      | -0.67                 | 295.35 | 22                  |
| acetic acid        | CH <sub>3</sub> COOH                          | C1s (CH <sub>3</sub> )  | 290.97       | -0.58                 | 291.16                      | -0.39                 | 291.55 | 22                  |
| water              | H <sub>2</sub> O                              | O1s                     | 538.69       | -1.01                 | 539.34                      | -0.36                 | 539.7  | 16                  |
| ozone              | O <sub>3</sub>                                | O1s middle              | 546.06       | -0.38                 | 546.74                      | 0.30                  | 546.44 | 23                  |
| ozone              | O <sub>3</sub>                                | O1s terminal            | 540.34       | -1.41                 | 541.53                      | -0.22                 | 541.75 | 23                  |
| oxygen             | O <sub>2</sub>                                | O1s weaker              | 542.84       | -1.36                 | 544.27                      | 0.07                  | 544.2  | 16                  |
| oxygen             | O <sub>2</sub>                                | O1s stronger            | 542.11       | -0.99                 | 543.11                      | 0.01                  | 543.1  | 16                  |
| nitrogen           | N <sub>2</sub>                                | N1s                     | 409.18       | -0.75                 | 409.78                      | -0.15                 | 409.93 | 17                  |
| ammonia            | NH <sub>3</sub>                               | N1s                     | 404.80       | -0.72                 | 405.07                      | -0.45                 | 405.52 | 19(17,20)           |
| hydrogen cyanide   | HCN                                           | N1s                     | 406.00       | -0.80                 | 406.90                      | 0.10                  | 406.8  | 19 (17,24)          |
| hydrogen cyanide   | HCN                                           | C1s                     | 292.90       | -0.60                 | 293.24                      | -0.26                 | 293.5  | 19                  |
| acetonitrile       | CH <sub>3</sub> CN                            | N1s                     | 404.67       | -0.91                 | 405.43                      | -0.15                 | 405.58 | 25                  |
| acetonitrile       | CH <sub>3</sub> CN                            | C1s (CH <sub>3</sub> )  | 292.16       | -0.73                 | 292.37                      | -0.51                 | 292.88 | 25                  |
| acetonitrile       | CH <sub>3</sub> CN                            | C1s (CN)                | 292.19       | -0.41                 | 292.33                      | -0.27                 | 292.60 | 25                  |
| glycine            | C <sub>2</sub> H <sub>5</sub> NO <sub>2</sub> | O1s (OH)                | 539.01       | -1.19                 | 539.55                      | -0.65                 | 540.2  | 26                  |
| glycine            | C <sub>2</sub> H <sub>5</sub> NO <sub>2</sub> | O1s (C=O)               | 537.06       | -1.34                 | 538.02                      | -0.38                 | 538.4  | 26                  |
| glycine            | C <sub>2</sub> H <sub>5</sub> NO <sub>2</sub> | N1s                     | 404.66       | -0.74                 | 405.10                      | -0.30                 | 405.4  | 26                  |
| glycine            | C <sub>2</sub> H <sub>5</sub> NO <sub>2</sub> | C1s (COOH)              | 294.47       | -0.73                 | 294.61                      | -0.59                 | 295.2  | 26                  |
| glycine            | C <sub>2</sub> H <sub>5</sub> NO <sub>2</sub> | C1s (CH <sub>2</sub> )  | 291.64       | -0.66                 | 292.00                      | -0.30                 | 292.3  | 26                  |
| pyridine           | C <sub>5</sub> H <sub>5</sub> N               | N1s                     | 403.88       | -0.94                 | 404.39                      | -0.43                 | 404.82 | 27                  |
| pyrrole            | C <sub>4</sub> H <sub>4</sub> NH              | N1s                     | 405.42       | -0.76                 | 405.82                      | -0.36                 | 406.18 | 27                  |
| aniline            | C <sub>6</sub> H <sub>5</sub> NH <sub>2</sub> | N1s                     | 404.53       | -0.78                 | 404.90                      | -0.41                 | 405.31 | 27                  |
| urea               | CO(NH <sub>2</sub> ) <sub>2</sub>             | O1s                     | 535.89       | -1.30                 | 536.61                      | -0.58                 | 537.19 | 19                  |
| urea               | CO(NH <sub>2</sub> ) <sub>2</sub>             | N1s                     | 405.32       | -0.77                 | 405.58                      | -0.51                 | 406.09 | 19                  |
| urea               | CO(NH <sub>2</sub> ) <sub>2</sub>             | C1s                     | 294.27       | -0.57                 | 294.22                      | -0.62                 | 294.84 | 19                  |
| methylamine        | CH <sub>3</sub> NH <sub>2</sub>               | N1s                     | 404.37       | -0.80                 | 404.82                      | -0.35                 | 405.17 | 19 (17,20)          |
| nitrobenzene       | C <sub>6</sub> H <sub>5</sub> NO <sub>2</sub> | O1s                     | 537.26       | -1.37                 | 538.05                      | -0.58                 | 538.63 | 19                  |
| nitrobenzene       | C <sub>6</sub> H <sub>5</sub> NO <sub>2</sub> | N1s                     | 410.85       | -0.75                 | 410.98                      | -0.62                 | 411.6  | 16                  |
| nitrobenzene       | C <sub>6</sub> H <sub>5</sub> NO <sub>2</sub> | C1s (C1)                | 291.43       | -0.65                 | 291.65                      | -0.43                 | 292.08 | 19                  |

**Table S5:** Continued

| name            | formula                                       | core level | $\Delta$ SCF |                       | evGW <sub>0</sub> @PBE(pre) |                       | BE     | Ref <sub>Exp.</sub> |
|-----------------|-----------------------------------------------|------------|--------------|-----------------------|-----------------------------|-----------------------|--------|---------------------|
|                 |                                               |            | BE           | $\Delta_{\text{exp}}$ | BE                          | $\Delta_{\text{exp}}$ |        |                     |
| nitrobenzene    | C <sub>6</sub> H <sub>5</sub> NO <sub>2</sub> | C1s (C2-4) | 290.47       | -0.66                 | 290.74                      | -0.39                 | 291.13 | 19                  |
| benzene         | C <sub>6</sub> H <sub>6</sub>                 | C1s        | 289.69       | -0.70                 | 290.13                      | -0.25                 | 290.38 | 28                  |
| phenylacetylene | C <sub>8</sub> H <sub>6</sub>                 | C1s (C3)   | 290.46       | -0.42                 | 290.83                      | -0.05                 | 290.88 | 29                  |
| phenylacetylene | C <sub>8</sub> H <sub>6</sub>                 | C1s (C2)   | 290.06       | -0.49                 | 290.39                      | -0.16                 | 290.55 | 29                  |
| phenylacetylene | C <sub>8</sub> H <sub>6</sub>                 | C1s (C4-6) | 289.73       | -0.43                 | 290.19                      | 0.03                  | 290.16 | 29                  |
| phenylacetylene | C <sub>8</sub> H <sub>6</sub>                 | C1s (C1)   | 289.36       | -0.39                 | 289.80                      | 0.05                  | 289.75 | 29                  |

## 6 Atomic corrections for hybrid functionals

**Table S6:** Atomic corrections  $\Delta\epsilon_{1s,\text{at}}^{\text{SKS}}$  in electronvolts as a function of  $\alpha$  for PBEh( $\alpha$ ) exchange-correlation functional for 2nd period elements B-F. The  $\alpha = 0$  value is repeated here for ease of comparison.

| $\alpha$ | B1s     | C1s     | N1s     | O1s     | F1s     |
|----------|---------|---------|---------|---------|---------|
| 0        | -0.0502 | -0.1176 | -0.2355 | -0.4244 | -0.7080 |
| 0.25     | -0.0534 | -0.1235 | -0.2451 | -0.4387 | -0.7281 |
| 0.5      | -0.0567 | -0.1295 | -0.2549 | -0.4532 | -0.7483 |

## 7 Pre-correction scheme

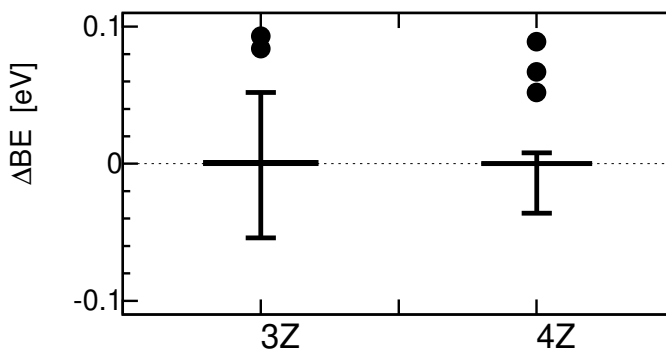**Figure S2:** Difference between pre- and post-corrected evGW<sub>0</sub>@PBE binding energies for the 65 1s excitations. The shaded region (which is collapsed to a line) contains 50% of the values, and the whiskers extend to encompass the 95% of the values. Outliers are shown as solid spheres. The difference is defined as the  $\Delta\text{BE} = \text{BE}_{i,\text{pre}} - \text{BE}_{i,\text{post}}$ .

# References

- (1) Blum, V.; Gehrke, R.; Hanke, F.; Havu, P.; Havu, V.; Ren, X.; Reuter, K.; Scheffler, M. Ab initio molecular simulations with numeric atom-centered orbitals. *Comput. Phys. Commun.* **2009**, *180*, 2175–2196.
- (2) Halkier, A.; Helgaker, T.; Jørgensen, P.; Klopper, W.; Koch, H.; Olsen, J.; Wilson, A. K. Basis-set convergence in correlated calculations on Ne, N<sub>2</sub>, and H<sub>2</sub>O. *Chem. Phys. Lett.* **1998**, *286*, 243–252.
- (3) Shih, B. C.; Xue, Y.; Zhang, P.; Cohen, M. L.; Louie, S. G. Quasiparticle band gap of ZnO: High accuracy from the conventional  $G^0W^0$  approach. *Phys. Rev. Lett.* **2010**, *105*, 1–4.
- (4) Friedrich, C.; Müller, M. C.; Blügel, S. Band convergence and linearization error correction of all-electron *GW* calculations: The extreme case of zinc oxide. *Phys. Rev. B* **2011**, *83*, 8–11.
- (5) Bruneval, F. Ionization energy of atoms obtained from *GW* self-energy or from random phase approximation total energies. *J. Chem. Phys.* **2012**, *136*, 194107.
- (6) Dunning, T. H. Gaussian basis sets for use in correlated molecular calculations. I. The atoms boron through neon and hydrogen. *J. Chem. Phys.* **1989**, *90*, 1007–1023.
- (7) Wilson, A. K.; van Mourik, T.; Dunning, T. H. Gaussian basis sets for use in correlated molecular calculations. VI. Sextuple zeta correlation consistent basis sets for boron through neon. *J. Mol. Struct. (Theochem)* **1996**, *388*, 339–349.
- (8) Kendall, R. A.; Dunning, T. H.; Harrison, R. J. Electron affinities of the first-row atoms revisited. Systematic basis sets and wave functions. *J. Chem. Phys.* **1992**, *96*, 6796–6806.
- (9) Woon, D. E.; Dunning, T. H. Gaussian basis sets for use in correlated molecular calculations. V. Core-valence basis sets for boron through neon. *J. Chem. Phys.* **1995**, *103*, 4572–4585.
- (10) Zhang, I. Y.; Ren, X.; Rinke, P.; Blum, V.; Scheffler, M. Numeric atom-centered-orbital basis sets with valence-correlation consistency from H to Ar. *New J. Phys.* **2013**, *15*.
- (11) Ambroise, M. A.; Jensen, F. Probing Basis Set Requirements for Calculating Core Ionization and Core Excitation Spectroscopy by the  $\Delta$  Self-Consistent-Field Approach. *J. Chem. Theory Comput.* **2019**, *15*, 325–337.
- (12) Kahk, J. M.; Lischner, J. Accurate absolute core-electron binding energies of molecules, solids, and surfaces from first-principles calculations. *Phys. Rev. Materials* **2019**, *3*, 100801.
- (13) Peng, B.; Lestranger, P. J.; Goings, J. J.; Caricato, M.; Li, X. Energy-Specific Equation-of-Motion Coupled-Cluster Methods for High-Energy Excited States: Application to K-edge X-ray Absorption Spectroscopy. *J. Chem. Theory Comput.* **2015**, *11*, 4146–4153.
- (14) Golze, D.; Keller, L.; Rinke, P. Accurate Absolute and Relative Core-Level Binding Energies from *GW*. *J. Phys. Chem. Lett.* **2020**, *11*, 1840–1847.
- (15) Myrseth, V.; Bozek, J. D.; Kukk, E.; Sæthre, L. J.; Thomas, T. D. Adiabatic and vertical carbon 1s ionization energies in representative small molecules. *J. Electron Spectrosc. Relat. Phenom.* **2002**, *122*, 57–63.
- (16) Siegbahn, K.; Nordling, C.; Johansson, G.; Hedman, J.; Hedén, P. F.; Hamrin, K.; Gelius, U.; Bergmark, T.; Werme, L. O.; Manne, R.; Baer, Y. *ESCA applied to free molecules*; North-Holland Publishing Company Amsterdam-London, 1969; p 12.
- (17) Thomas, T. D.; Shaw, R. W. Accurate core ionization potentials and photoelectron kinetic energies for light elements. *J. Electron Spectrosc. Relat. Phenom.* **1974**, *5*, 1081–1094.
- (18) Thomas, T. D. X-ray photoelectron spectroscopy of halomethanes. *J. Am. Chem. Soc.* **1970**, *92*, 4184–4189.
- (19) Bakke, A. A.; Chen, H.-W.; Jolly, W. L. A table of absolute core-electron binding-energies for gaseous atoms and molecules. *J. Electron Spectrosc. Relat. Phenom.* **1980**, *20*, 333–366.
- (20) Mills, B. E.; Martin, R. L.; Shirley, D. A. Further studies of the core binding energy-proton affinity correlation in molecules. *J. Am. Chem. Soc.* **1976**, *98*, 2380–2385.
- (21) Drake, J. E.; Riddle, C.; Henderson, H. E.; Glavinčevski, B. ESCA investigations of Group IV derivatives. Part III. Binding energies for methyl substituted disilyl and digermyl chalcogenide series. *Can. J. Chem.* **1977**, *55*, 2957–2961.
- (22) Naves de Brito, A.; Correia, N.; Svensson, S.; Ågren, H. A theoretical study of x-ray photoelectron spectra of model molecules for polymethylmethacrylate. *J. Chem. Phys.* **1991**, *95*, 2965–2974.
- (23) Mocellin, A.; Wiesner, K.; Sorensen, S. L.; Miron, C.; Guen, K. L.; Céolin, D.; Simon, M.; Morin, P.; Machado, A. B.; Björneholm, O.; Naves de Brito, A. Site selective dissociation upon core ionization of ozone. *Chem. Phys. Lett.* **2007**, *435*, 214–218.
- (24) Finn, P.; Pearson, R. K.; Hollander, J. M.; Jolly, W. L. Chemical shifts in core electron binding energies for some gaseous nitrogen compounds. *Inorg. Chem.* **1971**, *10*, 378–381.
- (25) Naves de Brito, A.; Svensson, S.; Ågren, H.; Delhalle, J. Experimental and theoretical study of the XPS core levels of gas phase acetonitrile, acrylonitrile and propionitrile. Model molecules for polyacrylonitrile. *J. Electron Spectrosc. Relat. Phenom.* **1993**, *63*, 239–251.
- (26) Plekan, O.; Feyer, V.; Richter, R.; Coreno, M.; de Simone, M.; Prince, K. C.; Carravetta, V. Investigation of the Amino Acids Glycine, Proline, and Methionine by Photoemission Spectroscopy. *J. Phys. Chem. A* **2007**, *111*, 10998–11005, PMID: 17918919.
- (27) Cavell, R. G.; Allison, D. A. Site of protonation in aromatic and acyclic amines and acyclic amides revealed by N1s core level electron spectroscopy. *J. Am. Chem. Soc.* **1977**, *99*, 4203–4204.
- (28) Myrseth, V.; Børve, K. J.; Thomas, T. D. The Substituent Effect of the Methyl Group. Carbon 1s Ionization Energies, Proton Affinities, and Reactivities of the Methylbenzenes. *J. Org. Chem.* **2007**, *72*, 5715–5723, PMID: 17595144.
- (29) Carravetta, V.; Iucci, G.; Ferri, A.; Russo, M. V.; Stranges, S.; de Simone, M.; Polzonetti, G. Synchrotron radiation photoemission study of some  $\pi$ -conjugated alkynes in the gas phase: Experiment and theory. *Chem. Phys.* **2001**, *264*, 175–186.
